# Supplementary material for: Quasioptical modeling of wave beams with and without mode conversion: I. Basic theory
Source: arXiv:1901.00268 ancillary file (2019-05-31)
Supplement: Supplementary file 1 [file supplement.pdf]

# Supplementary Material: Weyl calculus on a curved configuration space

Y. Zhou and I. Y. Dodin
*Princeton Plasma Physics Laboratory, Princeton, New Jersey 08543, USA*

This supplementary document summarizes the generalization of the Weyl calculus to a curved configuration space with an arbitrary given metric diffeomorphic to $\mathbb{R}^n$. Elements of this theory can also be found in Refs. [1, 2], and a detailed formulation of the Weyl calculus for a Euclidean configuration space is discussed in detail, for example, in Refs. [3, 4].

## I. BASIC DEFINITIONS

### A. State vectors and operators

Let us consider an $n$-dimensional configuration space $M^n$ with coordinates $\mathbf{x} \equiv \{x^0, x^1, \ldots, x^{n-1}\}$ and some metric $\boldsymbol{g}(\mathbf{x})$. We assume that $M^n$ is diffeomorphic to $\mathbb{R}^n$, namely, the $n$-dimensional Euclidean space or pseudo-Euclidean space with the same metric signature. Let us also consider scalar fields on this space and linear operators acting on them. An operator $\widehat{A}$ maps a given field $\Psi$ to a new field $\widehat{A}\Psi$ that can be expressed as follows:

$$(\widehat{A}\Psi)(\mathbf{x}) \doteq \int \mathrm{d}^n x' [g(\mathbf{x}')]^{1/2} \mathsf{A}(\mathbf{x}, \mathbf{x}')\Psi(\mathbf{x}'). \tag{1}$$

Here $\doteq$ denotes a definition; the integral is taken over $\mathbb{R}^n$ (and so are all integrals below, up to dimension); $g \doteq |\det \boldsymbol{g}|$; and $\mathsf{A}$ is some kernel function that determines $\widehat{A}$.

Consider also a family of all unitary operators $\widehat{A}_u$, which is a subset of all possible $\widehat{A}$. For a given $\Psi$, all image functions $\widehat{A}_u\Psi$ are mutually equivalent up to an isomorphism, so their family $\{\widehat{A}_u\Psi\}$ can be viewed as a single object, a "state vector" $|\Psi\rangle$, which belongs to a Hilbert space $\mathcal{H}$ with inner product

$$\langle\Psi|\Phi\rangle = \int \mathrm{d}^n x\, [g(\mathbf{x})]^{1/2}\, \Psi^*(\mathbf{x})\Phi(\mathbf{x}). \tag{2}$$

Then, Eq. (1) can be viewed as the "$\mathbf{x}$ representation" of $\widehat{A}$ (also see Sec. I D), while the operator itself can be understood more generally as a transformation of $|\Psi\rangle$, i.e., of the whole family $\{\widehat{A}_u\Psi\}$.

### B. Coordinate and momentum operators

Let us define the coordinate and momentum operators

$$\widehat{\mathbf{x}} = \{\widehat{x}^0, \widehat{x}^1, \ldots, \widehat{x}^{n-1}\}, \tag{3}$$

$$\widehat{\mathbf{p}} = \{\widehat{p}_0, \widehat{p}_1, \ldots, \widehat{p}_{n-1}\} \tag{4}$$

such that the $\mathbf{x}$ representations of $\widehat{x}^\mu$ and $\widehat{p}_\mu$ be as follows:

$$\widehat{x}^\mu\Psi = x^\mu\Psi, \tag{5}$$

$$\widehat{p}_\mu\Psi = -ig^{-1/4}\partial_\mu(g^{1/4}\Psi). \tag{6}$$

Here $\partial_\mu \doteq \partial/\partial x^\mu$, $x^\mu$ and $p_\mu$ are the corresponding eigenvalues, and the factor $g^{\pm 1/4}$ is introduced to keep $\widehat{\mathbf{p}}$ self-adjoint under the inner product (2) [5]. (This would not be the case if $M^n$ were not diffeomorphic to $\mathbb{R}^n$ [6].) Since $\widehat{p}_\mu = -i\partial_\mu - (i/4)[\partial_\mu(\ln g)]$, where the second term is simply a function of $\mathbf{x}$, the coordinate and momentum operators have the usual commutator

$$[\widehat{x}^\mu, \widehat{p}_\nu] = i\delta^\mu_\nu. \tag{7}$$

As can be checked by comparing Eqs. (5) and (6) with Eq. (1), the kernels $\mathsf{x}^\mu$ and $\mathsf{p}_\mu$ of the coordinate and momentum operators can be expressed as follows:

$$\mathsf{x}^\mu(\mathbf{x}_1, \mathbf{x}_2) = \frac{1}{2}\,(x_1^\mu + x_2^\mu)\,\delta(\mathbf{x}_1 - \mathbf{x}_2)\,\mathfrak{G}(\mathbf{x}_1, \mathbf{x}_2), \tag{8}$$

$$\mathsf{p}_\mu(\mathbf{x}_1, \mathbf{x}_2) = -i\,\frac{\partial\delta(\mathbf{x}_1 - \mathbf{x}_2)}{\partial x_1^\mu}\,\mathfrak{G}(\mathbf{x}_1, \mathbf{x}_2). \tag{9}$$

Here we introduced the function

$$\mathfrak{G}(\mathbf{x}_1, \mathbf{x}_2) \doteq [g(\mathbf{x}_1)g(\mathbf{x}_2)]^{-1/4}, \tag{10}$$

which is unity if the configuration space is Euclidean or pseudo-Euclidean ($g = 1$). We shall also use

$$\widehat{z} \doteq (\widehat{\mathbf{x}}, \widehat{\mathbf{p}}), \quad \zeta \wedge \widehat{z} \doteq \mathbf{q}\cdot\widehat{\mathbf{x}} - \mathbf{s}\cdot\widehat{\mathbf{p}}, \tag{11}$$

where $\zeta \doteq (\mathbf{s}, \mathbf{q})$, $\mathbf{a}\cdot\mathbf{b} \doteq a_\mu b^\mu$ for any $\mathbf{a}$ and $\mathbf{b}$, and summation over repeated indices is assumed as usual.

### C. Eigenvectors of $\widehat{\mathbf{x}}$ and $\widehat{\mathbf{p}}$

Let us consider the eigenvectors $|\mathbf{x}\rangle$ and $|\mathbf{p}\rangle$ of the coordinate and momentum operators, which are defined as

$$\widehat{\mathbf{x}}\,|\mathbf{x}\rangle = \mathbf{x}\,|\mathbf{x}\rangle\,, \quad \widehat{\mathbf{p}}\,|\mathbf{p}\rangle = \mathbf{p}\,|\mathbf{p}\rangle\,. \tag{12}$$

Since the operators $\widehat{\mathbf{x}}$ and $\widehat{\mathbf{p}}$ are self-adjoint, these eigenvectors can be chosen as mutually orthogonal, and we shall assume the following normalization:

$$\langle\mathbf{x}_1|\mathbf{x}_2\rangle = \mathfrak{G}(\mathbf{x}_1, \mathbf{x}_2)\,\delta(\mathbf{x}_1 - \mathbf{x}_2), \tag{13}$$

$$\langle\mathbf{p}_1|\mathbf{p}_2\rangle = \bar{\mathfrak{G}}(\mathbf{p}_1, \mathbf{p}_2)\,\delta(\mathbf{p}_1 - \mathbf{p}_2). \tag{14}$$

Here, we introduce $\bar{\mathfrak{G}}$ by analogy with $\mathfrak{G}$ as

$$\bar{\mathfrak{G}}(\mathbf{p}_1, \mathbf{p}_2) \doteq [\bar{g}(\mathbf{p}_1)\bar{g}(\mathbf{p}_2)]^{-1/4}. \tag{15}$$

The function $\bar{g}$ plays a role similar to that of $g$ in the equations below, but note that this is just an arbitrary

positive normalization factor introduced to maintain the symmetry between $\hat{\mathbf{x}}$ and $\hat{\mathbf{p}}$ [7]. Then,

$$\int \mathrm{d}^n x\, [g(\mathbf{x})]^{1/2}\, |\mathbf{x}\rangle\, \langle\mathbf{x}| = \hat{\mathbb{1}}, \tag{16}$$

$$\int \mathrm{d}^n p\, [\bar{g}(\mathbf{p})]^{1/2}\, |\mathbf{p}\rangle\, \langle\mathbf{p}| = \hat{\mathbb{1}} \tag{17}$$

(here $\hat{\mathbb{1}}$ is the unit operator), and likewise,

$$\int \mathrm{d}^n x\, [g(\mathbf{x})]^{1/2}\, |\mathbf{x}\rangle\, \mathbf{x}\, \langle\mathbf{x}| = \hat{\mathbf{x}}, \tag{18}$$

$$\int \mathrm{d}^n p\, [\bar{g}(\mathbf{p})]^{1/2}\, |\mathbf{p}\rangle\, \mathbf{p}\, \langle\mathbf{p}| = \hat{\mathbf{p}}. \tag{19}$$

Also note that the trace of any operator can be written as

$$\begin{aligned}\operatorname{tr}\hat{A} &= \operatorname{tr}\int \mathrm{d}^n x\, [g(\mathbf{x})]^{1/2}\, |\mathbf{x}\rangle\, \langle\mathbf{x}|\, \hat{A} \\ &= \int \mathrm{d}^n x\, [g(\mathbf{x})]^{1/2}\, \langle\mathbf{x}|\hat{A}|\mathbf{x}\rangle\,,\end{aligned} \tag{20}$$

and similarly through an integral over the $\mathbf{p}$ space.

### D. Representations of state vectors and operators

Let $\xi(\mathbf{x};\mathbf{x}')$ be the coordinate representation of $|\mathbf{x}'\rangle$ for a given $\mathbf{x}'$. On one hand, $\xi(\mathbf{x};\mathbf{x}')$ is an eigenfunction of $\hat{\mathbf{x}}$ corresponding to the eigenvalue $\mathbf{x}'$, so $\hat{\mathbf{x}}\xi(\mathbf{x};\mathbf{x}') = \mathbf{x}'\xi(\mathbf{x};\mathbf{x}')$. On the other hand, like any other field, $\xi(\mathbf{x};\mathbf{x}')$ satisfies Eq. (5), so $\hat{\mathbf{x}}\xi(\mathbf{x};\mathbf{x}') = \mathbf{x}\xi(\mathbf{x};\mathbf{x}')$. Therefore, $(\mathbf{x}-\mathbf{x}')\xi(\mathbf{x};\mathbf{x}') = 0$, which means that $\xi$ is delta-shaped, $\xi(\mathbf{x};\mathbf{x}') = \alpha(\mathbf{x}')\delta(\mathbf{x}-\mathbf{x}')$. From Eq. (13) combined with Eq. (2), one finds that $|\alpha(\mathbf{x})|^2 g(\mathbf{x}) = 1$. Hence, we adopt $\alpha(\mathbf{x}) = |g(\mathbf{x})|^{-1/2}$, which leads to

$$\xi(\mathbf{x};\mathbf{x}') = [g(\mathbf{x})]^{-1/2}\delta(\mathbf{x}-\mathbf{x}'). \tag{21}$$

Then, Eq. (2) readily yields

$$\langle\mathbf{x}|\Psi\rangle = \Psi(\mathbf{x}). \tag{22}$$

Similarly,

$$\begin{aligned}\langle\mathbf{x}_1|\hat{A}|\mathbf{x}_2\rangle &= (\hat{A}\,|\mathbf{x}_2\rangle)(\mathbf{x}_1) \\ &= \int \mathrm{d}^n x'\, [g(\mathbf{x}')]^{1/2}\mathsf{A}(\mathbf{x}_1,\mathbf{x}')\xi(\mathbf{x}';\mathbf{x}_2) \\ &= \int \mathrm{d}^n x'\, \mathsf{A}(\mathbf{x}_1,\mathbf{x}')\delta(\mathbf{x}'-\mathbf{x}_2) \\ &= \mathsf{A}(\mathbf{x}_1,\mathbf{x}_2),\end{aligned} \tag{23}$$

and Eq. (20) also gives

$$\operatorname{tr}\hat{A} = \int \mathrm{d}^n x\, [g(\mathbf{x})]^{1/2}\mathsf{A}(\mathbf{x},\mathbf{x}). \tag{24}$$

Next, from Eq. (22), we determine that $\eta(\mathbf{x};\mathbf{p}') \doteq \langle\mathbf{x}|\mathbf{p}'\rangle$ is the $\mathbf{x}$ representation of the momentum-operator eigenvector corresponding to the eigenvalue $\mathbf{p}'$. Then, by solving the equation $\hat{\mathbf{p}}\eta(\mathbf{x};\mathbf{p}') = \mathbf{p}'\eta(\mathbf{x};\mathbf{p}')$ with $\hat{\mathbf{p}}$ given by Eq. (6), one obtains

$$\eta(\mathbf{x};\mathbf{p}') = \frac{\exp(i\mathbf{p}'\cdot\mathbf{x})}{(2\pi)^{n/2}[g(\mathbf{x})\bar{g}(\mathbf{p}')]^{1/4}}, \tag{25}$$

where we used Eq. (14) and, like in the case with $\xi(\mathbf{x};\mathbf{x}')$, assumed a certain (zero) constant phase. Hence,

$$\langle\mathbf{x}|\mathbf{p}\rangle = \langle\mathbf{p}|\mathbf{x}\rangle^* = \frac{\exp(i\mathbf{p}\cdot\mathbf{x})}{(2\pi)^{n/2}[g(\mathbf{x})\bar{g}(\mathbf{p})]^{1/4}}. \tag{26}$$

Likewise, $\langle\mathbf{p}|\mathbf{x}\rangle$ is the $\mathbf{p}$ representation of the coordinate-operator eigenvector corresponding to the eigenvalue $\mathbf{x}$, and $\langle\mathbf{p}|\Psi\rangle$ is the $\mathbf{p}$ representation of $|\Psi\rangle$. The $\mathbf{p}$ representations of the operators can be introduced similarly.

## II. HEISENBERG GENERATING OPERATOR

Consider the following operators:

$$\hat{T}_{\mathbf{s}} \doteq \exp(-i\mathbf{s}\cdot\hat{\mathbf{p}}), \quad \hat{T}_{\mathbf{q}} \doteq \exp(i\mathbf{q}\cdot\hat{\mathbf{x}}). \tag{27}$$

They can be understood as the *operators of translation* in the $\mathbf{x}$ and $\mathbf{p}$ spaces, respectively, in the sense that

$$\begin{aligned}\hat{T}_{\mathbf{s}}\,|\mathbf{x}\rangle &= \int \mathrm{d}^n p\, [\bar{g}(\mathbf{p})]^{1/2} e^{-i\mathbf{s}\cdot\hat{\mathbf{p}}}\, |\mathbf{p}\rangle\, \langle\mathbf{p}|\mathbf{x}\rangle \\ &= [g(\mathbf{x}+\mathbf{s})/g(\mathbf{x})]^{1/4}\int \mathrm{d}^n p\, [\bar{g}(\mathbf{p})]^{1/2}\, |\mathbf{p}\rangle\, \langle\mathbf{p}|\mathbf{x}+\mathbf{s}\rangle \\ &= [g(\mathbf{x}+\mathbf{s})/g(\mathbf{x})]^{1/4}\, |\mathbf{x}+\mathbf{s}\rangle\end{aligned} \tag{28}$$

[here we used Eq. (26)] and, similarly,

$$\hat{T}_{\mathbf{q}}\,|\mathbf{p}\rangle = [\bar{g}(\mathbf{p}+\mathbf{q})/\bar{g}(\mathbf{p})]^{1/4}\, |\mathbf{p}+\mathbf{q}\rangle\,. \tag{29}$$

Let us also define the *Heisenberg generating operator*

$$\hat{T}_\zeta \doteq \exp(-i\zeta\wedge\hat{z}). \tag{30}$$

Using the Baker–Campbell–Hausdorff formula,

$$e^{\hat{A}}e^{\hat{B}} = e^{\hat{A}+\hat{B}+[\hat{A},\hat{B}]/2} \tag{31}$$

(where it is assumed that both $\hat{A}$ and $\hat{B}$ commute with their commutator $[\hat{A},\hat{B}]$) and Eq. (7), one can show that

$$\hat{T}_{\zeta_1+\zeta_2} = \hat{T}_{\zeta_1}\hat{T}_{\zeta_2}e^{-i\zeta_1\wedge\zeta_2/2}, \tag{32}$$

and as a special case,

$$\hat{T}_\zeta = \hat{T}_{-\mathbf{s}}\hat{T}_{-\mathbf{q}}e^{i\mathbf{s}\cdot\mathbf{q}/2} = \hat{T}_{-\mathbf{q}}\hat{T}_{-\mathbf{s}}e^{-i\mathbf{s}\cdot\mathbf{q}/2}. \tag{33}$$

Subsequently, the $\mathbf{x}$ representation of $\hat{T}_\zeta$ reads

$$\begin{aligned}\mathsf{T}_\zeta(\mathbf{x}_1,&\mathbf{x}_2) \\ &= \langle\mathbf{x}_1|\hat{T}_{-\mathbf{q}}\hat{T}_{-\mathbf{s}}e^{-i\mathbf{s}\cdot\mathbf{q}/2}|\mathbf{x}_2\rangle \\ &= [g(\mathbf{x}_2-\mathbf{s})/g(\mathbf{x}_2)]^{1/4}e^{-i\mathbf{q}\cdot(\mathbf{x}_1+\mathbf{s}/2)}\,\langle\mathbf{x}_1|\mathbf{x}_2-\mathbf{s}\rangle \\ &= \mathfrak{G}(\mathbf{x}_1,\mathbf{x}_2)\,\delta(\mathbf{x}_1-\mathbf{x}_2+\mathbf{s})\,e^{-i\mathbf{q}\cdot(\mathbf{x}_1+\mathbf{s}/2)},\end{aligned} \tag{34}$$

so in particular, one obtains [cf. Eq. (24)]

$$\operatorname{tr}\hat{T}_\zeta = (2\pi)^n\delta(\zeta). \tag{35}$$

## III. WIGNER OPERATOR

Next, let us define the *Wigner operator* as the Fourier transform of the Heisenberg generating operator,

$$\widehat{\Delta}_z \doteq \int \frac{\mathrm{d}^{2n}\zeta}{(2\pi)^n}\, \widehat{T}_\zeta e^{i\zeta\wedge z}, \tag{36}$$

where $z \doteq (\mathbf{x}, \mathbf{p})$ is a $2n$-dimensional "phase space" coordinate that serves as a parameter. The Wigner operators with different $z$ are orthogonal in the sense that

$$\begin{aligned}
\mathrm{tr}\,(\widehat{\Delta}_z\widehat{\Delta}_{z'}) &= \int \frac{\mathrm{d}^{2n}\zeta\,\mathrm{d}^{2n}\zeta'}{(2\pi)^{2n}}\,\mathrm{tr}\,(\widehat{T}_\zeta\widehat{T}_{\zeta'})\, e^{i(\zeta\wedge z+\zeta'\wedge z')} \\
&= \int \frac{\mathrm{d}^{2n}\zeta\,\mathrm{d}^{2n}\zeta'}{(2\pi)^{2n}}\,\mathrm{tr}\,\widehat{T}_{\zeta+\zeta'}\, e^{i(\zeta\wedge z+\zeta'\wedge z'+\zeta\wedge\zeta'/2)} \\
&= \int \frac{\mathrm{d}^{2n}\zeta}{(2\pi)^n}\, e^{i\zeta\wedge(z-z')} \\
&= (2\pi)^n\delta(z-z'),
\end{aligned} \tag{37}$$

where Eqs. (32) and (35) are used. Also,

$$\begin{aligned}
\int \frac{\mathrm{d}^{2n}z}{(2\pi)^n}\,\widehat{\Delta}_z &= \int \frac{\mathrm{d}^{2n}\zeta\,\mathrm{d}^{2n}z}{(2\pi)^{2n}}\,\widehat{T}_\zeta e^{i\zeta\wedge z} \\
&= \int \mathrm{d}^{2n}\zeta\,\widehat{T}_\zeta\delta(\zeta) = \widehat{\mathbb{1}}.
\end{aligned} \tag{38}$$

From Eq. (34), the $\mathbf{x}$ representation of $\widehat{\Delta}_z$ is

$$\begin{aligned}
\Delta_z(\mathbf{x}_1,\mathbf{x}_2) &\doteq \langle\mathbf{x}_1|\widehat{\Delta}_z|\mathbf{x}_2\rangle \\
&= \int \frac{\mathrm{d}^{2n}\zeta}{(2\pi)^n}\,\mathsf{T}_\zeta(\mathbf{x}_1,\mathbf{x}_2)e^{i\zeta\wedge z} \\
&= \int \frac{\mathrm{d}^{2n}\zeta}{(2\pi)^n}\,\frac{\delta(\mathbf{x}_1-\mathbf{x}_2+\mathbf{s})}{[g(\mathbf{x}_1)g(\mathbf{x}_2)]^{1/4}}\,e^{-i\mathbf{s}\cdot\mathbf{p}-i\mathbf{q}\cdot(\mathbf{x}_1+\mathbf{s}/2-\mathbf{x})} \\
&= \int \mathrm{d}^n s\,\frac{\delta(\mathbf{x}_1-\mathbf{x}_2+\mathbf{s})\delta(\mathbf{x}-\mathbf{x}_1-\mathbf{s}/2)}{[g(\mathbf{x}_1)g(\mathbf{x}_2)]^{1/4}}\,e^{-i\mathbf{s}\cdot\mathbf{p}}.
\end{aligned} \tag{39}$$

Note that this can be further simplified as follows:

$$\Delta_z(\mathbf{x}_1,\mathbf{x}_2) = \mathfrak{G}(\mathbf{x}_1,\mathbf{x}_2)\,\delta[\mathbf{x}-(\mathbf{x}_1+\mathbf{x}_2)/2]e^{i(\mathbf{x}_1-\mathbf{x}_2)\cdot\mathbf{p}}. \tag{40}$$

Also note that Eq. (39) can be used to obtain the following alternative representation of $\widehat{\Delta}_z$:

$$\begin{aligned}
\widehat{\Delta}_z &= \int \mathrm{d}^n x_1\mathrm{d}^n x_2\,[g(\mathbf{x}_1)g(\mathbf{x}_2)]^{1/2}\,|\mathbf{x}_1\rangle\,\Delta_z(\mathbf{x}_1,\mathbf{x}_2)\,\langle\mathbf{x}_2| \\
&= \int \mathrm{d}^n s\,\mathrm{d}^n x_1\,\frac{\delta(\mathbf{x}-\mathbf{x}_1-\mathbf{s}/2)\,|\mathbf{x}_1\rangle\,\langle\mathbf{x}_1+\mathbf{s}|}{[g(\mathbf{x}_1)g(\mathbf{x}_1+\mathbf{s})]^{-1/4}}\,e^{-i\mathbf{s}\cdot\mathbf{p}} \\
&= \int \mathrm{d}^n s\,G(\mathbf{x},\mathbf{s})\,|\mathbf{x}-\mathbf{s}/2\rangle\,\langle\mathbf{x}+\mathbf{s}/2|\,e^{-i\mathbf{s}\cdot\mathbf{p}},
\end{aligned} \tag{41}$$

where we introduced

$$G(\mathbf{x},\mathbf{s}) \doteq [g(\mathbf{x}-\mathbf{s}/2)g(\mathbf{x}+\mathbf{s}/2)]^{1/4}. \tag{42}$$

Like $\mathfrak{G}$, the function $G$ is equal to one if the $\mathbf{x}$ space is Euclidean or pseudo-Euclidean. Unlike in $\mathfrak{G}$, the power index in Eq. (42) is actually $+1/4$, not $-1/4$.

## IV. WIGNER–WEYL TRANSFORM

### A. Direct transform

With the Wigner operator, we can define the Wigner–Weyl transform $\mathscr{W}_z : \widehat{A} \mapsto A$, which maps any given operator $\widehat{A}$ defined on the Hilbert space $\mathcal{H}$ to a function $A$ ("Weyl symbol") on a $2n$-dimensional phase space $z$,

$$A(z) = \mathscr{W}_z[\widehat{A}] \doteq \mathrm{tr}\,(\widehat{\Delta}_z\widehat{A}). \tag{43}$$

Using Eq. (41), the Wigner–Weyl transform can also be expressed as follows:

$$A(z) = \int \mathrm{d}^n s\,G(\mathbf{x},\mathbf{s})\,\langle\mathbf{x}+\mathbf{s}/2|\widehat{A}|\mathbf{x}-\mathbf{s}/2\rangle\,e^{-i\mathbf{s}\cdot\mathbf{p}}. \tag{44}$$

Note that the phase-space integral of a Weyl symbol $A(z)$ equals the trace of its corresponding operator $\widehat{A}$,

$$\begin{aligned}
&\int \frac{\mathrm{d}^{2n}z}{(2\pi)^n}\,A(z) \\
&\quad= \int \mathrm{d}^n x\,\mathrm{d}^n s\,G(\mathbf{x},\mathbf{s})\,\langle\mathbf{x}+\mathbf{s}/2|\widehat{A}|\mathbf{x}-\mathbf{s}/2\rangle\,\delta(\mathbf{s}) \\
&\quad= \int \mathrm{d}^n x\,[g(\mathbf{x})]^{1/2}\,\langle\mathbf{x}|\widehat{A}|\mathbf{x}\rangle = \mathrm{tr}\,\widehat{A}.
\end{aligned} \tag{45}$$

Also, the Weyl symbol of the adjoint of any $\widehat{A}$ is the complex conjugate of the Weyl symbol of $\widehat{A}$ itself, since

$$\begin{aligned}
\mathscr{W}_z[\widehat{A}^\dagger] &= \int \mathrm{d}^n s\,G(\mathbf{x},\mathbf{s})\,\langle\mathbf{x}+\mathbf{s}/2|\widehat{A}^\dagger|\mathbf{x}-\mathbf{s}/2\rangle\,e^{-i\mathbf{p}\cdot\mathbf{s}} \\
&= \int \mathrm{d}^n s\,G(\mathbf{x},\mathbf{s})\,\langle\mathbf{x}-\mathbf{s}/2|\widehat{A}|\mathbf{x}+\mathbf{s}/2\rangle^*\,e^{-i\mathbf{p}\cdot\mathbf{s}} \\
&= \int \mathrm{d}^n s\,G(\mathbf{x},-\mathbf{s})\,\langle\mathbf{x}+\mathbf{s}/2|\widehat{A}|\mathbf{x}-\mathbf{s}/2\rangle^*\,e^{i\mathbf{p}\cdot\mathbf{s}} \\
&= (\mathscr{W}_z[\widehat{A}])^*,
\end{aligned} \tag{46}$$

where we used the fact that $G(\mathbf{x},-\mathbf{s}) = G(\mathbf{x},\mathbf{s})$. In particular, this implies that the Weyl symbol of a self-adjoint operator on $\mathcal{H}$ is a real function.

### B. Inverse transform

The inverse Wigner–Weyl transform $\mathscr{W}^{-1} : A \mapsto \widehat{A}$ maps a given function $A(z)$ on phase space to the corresponding operator $\widehat{A}$ via

$$\widehat{A} = \mathscr{W}^{-1}[A(z)] \doteq \int \frac{\mathrm{d}^{2n}z}{(2\pi)^n}\,A(z)\widehat{\Delta}_z, \tag{47}$$

or equivalently, using Eq. (41),

$$\widehat{A} = \int \frac{\mathrm{d}^{2n}z\,\mathrm{d}^n s}{(2\pi)^n}\,G(\mathbf{x},\mathbf{s})\,A(z)\,|\mathbf{x}-\mathbf{s}/2\rangle\,\langle\mathbf{x}+\mathbf{s}/2|\,e^{-i\mathbf{s}\cdot\mathbf{p}}.$$

Equation (47) can be proven as follows. By substituting Eq. (44) into the right-hand side of Eq. (47), we obtain

$$\begin{aligned}\mathscr{W}^{-1}[A(z)] &= \frac{1}{(2\pi)^n}\int \mathrm{d}^{2n}z\,\mathrm{d}^n s\, G(\mathbf{x},\mathbf{s})\widehat{\Delta}_z e^{-i\mathbf{s}\cdot\mathbf{p}}\,\langle \mathbf{x}+\mathbf{s}/2|\widehat{A}|\mathbf{x}-\mathbf{s}/2\rangle \\ &= \frac{1}{(2\pi)^n}\int \mathrm{d}^{2n}z\,\mathrm{d}^n s\,\mathrm{d}^n x_1\,\mathrm{d}^n x_2\, G(\mathbf{x},\mathbf{s})[g(\mathbf{x}_1)g(\mathbf{x}_2)]^{1/2}\,|\mathbf{x}_1\rangle\,\Delta_z(\mathbf{x}_1,\mathbf{x}_2)\,\langle\mathbf{x}_2|\,e^{-i\mathbf{s}\cdot\mathbf{p}}\,\langle \mathbf{x}+\mathbf{s}/2|\widehat{A}|\mathbf{x}-\mathbf{s}/2\rangle\,. \end{aligned} \tag{48}$$

Then, using Eq. (40), we also obtain

$$\begin{aligned}&\mathscr{W}^{-1}[A(z)] \\ &= \frac{1}{(2\pi)^n}\int \mathrm{d}^{2n}z\,\mathrm{d}^n s\,\mathrm{d}^n x_1\,\mathrm{d}^n x_2\, G(\mathbf{x},\mathbf{s})[g(\mathbf{x}_1)g(\mathbf{x}_2)]^{1/4}\delta[\mathbf{x}-(\mathbf{x}_1+\mathbf{x}_2)/2]e^{i(\mathbf{x}_1-\mathbf{x}_2-\mathbf{s})\cdot\mathbf{p}}\,|\mathbf{x}_1\rangle\,\langle \mathbf{x}+\mathbf{s}/2|\widehat{A}|\mathbf{x}-\mathbf{s}/2\rangle\,\langle\mathbf{x}_2| \\ &= \int \mathrm{d}^n x\,\mathrm{d}^n s\,\mathrm{d}^n x_1\mathrm{d}^n x_2\, G(\mathbf{x},\mathbf{s})[g(\mathbf{x}_1)g(\mathbf{x}_2)]^{1/4}\delta[\mathbf{x}-(\mathbf{x}_1+\mathbf{x}_2)/2]\delta(\mathbf{x}_1-\mathbf{x}_2-\mathbf{s})\,|\mathbf{x}_1\rangle\,\langle \mathbf{x}+\mathbf{s}/2|\widehat{A}|\mathbf{x}-\mathbf{s}/2\rangle\,\langle\mathbf{x}_2| \\ &= \int \mathrm{d}^n x_1\mathrm{d}^n x_2\,[g(\mathbf{x}_1)g(\mathbf{x}_2)]^{1/2}\,|\mathbf{x}_1\rangle\,\langle\mathbf{x}_1|\widehat{A}|\mathbf{x}_2\rangle\,\langle\mathbf{x}_2| \\ &= \widehat{A}. \end{aligned} \tag{49}$$

As a consistency check, let us substitute Eq. (47) to the right-hand side of Eq. (43). Then, using Eq. (37), we obtain

$$\mathscr{W}_z[\widehat{A}] = \int \frac{\mathrm{d}^{2n}z'}{(2\pi)^n}\,A(z')\,\mathrm{tr}\,(\widehat{\Delta}_z\widehat{\Delta}_{z'}) = \int \mathrm{d}^{2n}z'\,A(z')\,\delta(z-z') = A(z). \tag{50}$$

### C. Weyl correspondence

The Wigner–Weyl transform (43) and the inverse Wigner–Weyl transform (47) set the (Weyl) correspondence $\widehat{A} \Leftrightarrow A(z)$ between operators on the Hilbert space $\mathcal{H}$ and functions on the phase space $z$. For example, as can be seen easily,

$$\mathscr{W}_z[\widehat{x}^\mu] = x^\mu. \tag{51}$$

Also, from Eqs. (9) and (44), we have

$$\begin{aligned}\mathscr{W}_z[\widehat{p}_\mu] &= \int \mathrm{d}^n s\,[-i\partial_\mu\delta(\mathbf{s})]e^{-i\mathbf{s}\cdot\mathbf{p}} \\ &= \int \mathrm{d}^n s\,\delta(\mathbf{s})p_\mu e^{-i\mathbf{s}\cdot\mathbf{p}} = p_\mu. \end{aligned} \tag{52}$$

More generally, it can be seen that

$$\mathscr{W}_z[f(\widehat{\mathbf{x}})] = f(\mathbf{x}), \quad \mathscr{W}_z[f(\widehat{\mathbf{p}})] = f(\mathbf{p}), \tag{53}$$

where $f$ is any function. Some other special cases of the Weyl correspondence are discussed in Sec. VI.

## V. MOYAL PRODUCT

The Weyl symbol of the product of two given linear operators $\widehat{A}$ and $\widehat{B}$ is given by the Moyal (star) product,

$$\begin{aligned}A(z)\star B(z) &\doteq \mathscr{W}_z[\widehat{A}\widehat{B}] = \mathrm{tr}\,(\widehat{\Delta}_z\widehat{A}\widehat{B}) \\ &= \int \frac{\mathrm{d}^{2n}z'\mathrm{d}^{2n}z''}{(2\pi)^{2n}}\,A(z')B(z'')\mathrm{tr}\,(\widehat{\Delta}_z\widehat{\Delta}_{z'}\widehat{\Delta}_{z''}). \end{aligned} \tag{54}$$

Using Eq. (36), we can rewrite this as follows:

$$\begin{aligned}\mathrm{tr}\,(\widehat{\Delta}_z\widehat{\Delta}_{z'}\widehat{\Delta}_{z''}) = \int \frac{\mathrm{d}^{2n}\zeta\,\mathrm{d}^{2n}\zeta'\mathrm{d}^{2n}\zeta''}{(2\pi)^{3n}}\,\mathrm{tr}\,(\widehat{T}_\zeta\widehat{T}_{\zeta'}\widehat{T}_{\zeta''}) \\ \times e^{i(\zeta\wedge z+\zeta'\wedge z'+\zeta''\wedge z'')}. \end{aligned} \tag{55}$$

From Eqs. (32) and (35), we have

$$\begin{aligned}\mathrm{tr}\,(\widehat{T}_\zeta\widehat{T}_{\zeta'}\widehat{T}_{\zeta''}) &= \mathrm{tr}\,(\widehat{T}_{\zeta+\zeta'+\zeta''})e^{i[\zeta\wedge(\zeta'+\zeta'')+\zeta'\wedge\zeta'']/2} \\ &= (2\pi)^n\delta(\zeta+\zeta'+\zeta'')e^{i\zeta'\wedge\zeta''/2}. \end{aligned} \tag{56}$$

Substituting into Eq. (55), we obtain

$$\begin{aligned}&\mathrm{tr}\,(\widehat{\Delta}_z\widehat{\Delta}_{z'}\widehat{\Delta}_{z''}) \\ &\quad= \int \frac{\mathrm{d}^{2n}\zeta'\mathrm{d}^{2n}\zeta''}{(2\pi)^{2n}}e^{i[\zeta'\wedge(z'-z+\zeta''/2)+\zeta''\wedge(z''-z)]} \\ &\quad= \int \mathrm{d}^{2n}\zeta''\delta(z'-z+\zeta''/2)e^{i\zeta''\wedge(z''-z)} \\ &\quad= 2^{2n}e^{-2i(z'-z)\wedge(z''-z)}. \end{aligned} \tag{57}$$

Hence, we arrive at the following integral form of the Moyal product:

$$\begin{aligned}&A(z)\star B(z) \\ &\quad= \int \frac{\mathrm{d}^{2n}z'\,\mathrm{d}^{2n}z''}{\pi^{2n}}A(z')B(z'')e^{-2i(z'-z)\wedge(z''-z)} \\ &\quad= \int \frac{\mathrm{d}^{2n}\zeta_1\mathrm{d}^{2n}\zeta_2}{\pi^{2n}}A(z+\zeta_1)B(z+\zeta_2)e^{-2i\zeta_1\wedge\zeta_2}. \end{aligned} \tag{58}$$

There also exists an alternative, pseudo-differential form of this product. In order to derive it, let us rewrite Eq. (58) as follows:

$$A(z)\star B(z) = \int \frac{\mathrm{d}^{2n}z'\,\mathrm{d}^{2n}\zeta}{(2\pi)^{2n}}\,A(z')B(z+\zeta/2)e^{i\zeta\wedge(z'-z)}.$$

Next, we Taylor-expand $B(z+\zeta/2)$ to obtain

$$B(z+\zeta/2)e^{i\zeta\wedge(z'-z)} = e^{i\zeta\wedge(z'-z)}\sum_{m=0}^{\infty}\left(\frac{\zeta}{2}\frac{\partial}{\partial z}\right)^m\frac{B(z)}{m!}.$$

Here, the derivative acts on $B(z)$, which we denote as $\overrightarrow{\partial}_z$. Also, $\zeta$ can be replaced with derivatives acting on the exponential to the left, which we denote as $\overleftarrow{\partial}_z$:

$$e^{i\zeta\wedge(z'-z)}\left(\zeta\overrightarrow{\partial}_z\right)^m = e^{i\zeta\wedge(z'-z)}\left(-i\overleftarrow{\partial}_z\wedge\overrightarrow{\partial}_z\right)^m. \tag{59}$$

Using this, we can rewrite the above formula as

$$\begin{aligned} B(z+\zeta/2)e^{i\zeta\wedge(z'-z)} &= e^{i\zeta\wedge(z'-z)}\widehat{\mathscr{Z}}B(z),\\ \widehat{\mathscr{Z}} \doteq \sum_{m=0}^{\infty}\frac{1}{m!}\left(\frac{i\widehat{\mathcal{L}}}{2}\right)^m &= \exp\left(\frac{i\widehat{\mathcal{L}}}{2}\right), \end{aligned} \tag{60}$$

where $\widehat{\mathcal{L}}$ is the Janus operator, namely,

$$\widehat{\mathcal{L}} \doteq \overleftarrow{\partial}_{\mathbf{x}}\cdot\overrightarrow{\partial}_{\mathbf{p}} - \overleftarrow{\partial}_{\mathbf{p}}\cdot\overrightarrow{\partial}_{\mathbf{x}} = -\overleftarrow{\partial}_z\wedge\overrightarrow{\partial}_z. \tag{61}$$

Subsequently, we obtain the pseudo-differential form of the Moyal product:

$$\begin{aligned} A(z)\star B(z) &= \int \frac{\mathrm{d}^{2n}z'\,\mathrm{d}^{2n}\zeta}{(2\pi)^{2n}}\,A(z')\left[e^{i\zeta\wedge(z'-z)}\widehat{\mathscr{Z}}B(z)\right]\\ &= \left[\int \mathrm{d}^{2n}z'\,A(z')\delta(z'-z)\right]\widehat{\mathscr{Z}}B(z)\\ &= A(z)\widehat{\mathscr{Z}}B(z), \end{aligned} \tag{62}$$

or more explicitly,

$$A(z)\star B(z) = A(z)\exp(i\widehat{\mathcal{L}}/2)B(z). \tag{63}$$

## VI. SOME SPECIAL CASES OF THE WEYL CORRESPONDENCE

Using the Moyal product, let us also derive some other special cases of the Weyl correspondence that are of practical interest. As should become clear from these calculations, the Weyl symbol of an operator that is *any* given combination $f(\widehat{\mathbf{x}},\widehat{\mathbf{p}})$ of $\widehat{\mathbf{x}}$ and $\widehat{\mathbf{p}}$ approaches $f(\mathbf{x},\mathbf{p})$ in the "geometrical-optics" limit, when the commutator $[\widehat{x}^\mu,\widehat{p}_\nu]$ is negligible. However, in general, $f(\widehat{\mathbf{x}},\widehat{\mathbf{p}})\neq f(\mathbf{x},\mathbf{p})$.

### A. $\mathscr{W}^{-1}[\mathbf{p}f(\mathbf{x})]$

For any $f$,

$$\begin{aligned} \mathscr{W}_z[\widehat{\mathbf{p}}f(\widehat{\mathbf{x}})] &= \mathbf{p}\star f(\mathbf{x})\\ &= \mathbf{p}\exp\left(-\frac{i}{2}\overleftarrow{\partial}_{\mathbf{p}}\cdot\overrightarrow{\partial}_{\mathbf{x}}\right)f(\mathbf{x})\\ &= \mathbf{p}f(\mathbf{x}) - \frac{i}{2}\nabla f(\mathbf{x}). \end{aligned} \tag{64}$$

Likewise,

$$\mathscr{W}_z[f(\widehat{\mathbf{x}})\widehat{\mathbf{p}}] = \mathbf{p}f(\mathbf{x}) + \frac{i}{2}\nabla f(\mathbf{x}). \tag{65}$$

A comparison with Eq. (64) shows that the second terms are due to non-commutation of $\widehat{\mathbf{x}}$ and $\widehat{\mathbf{p}}$ and vanish when the commutator is negligible. Also, these formulas lead to

$$\widehat{\mathbf{p}}f(\widehat{\mathbf{x}}) = \mathscr{W}^{-1}[\mathbf{p}f(\mathbf{x})] - \frac{i}{2}(\nabla f)(\widehat{\mathbf{x}}), \tag{66}$$

$$f(\widehat{\mathbf{x}})\widehat{\mathbf{p}} = \mathscr{W}^{-1}[\mathbf{p}f(\mathbf{x})] + \frac{i}{2}(\nabla f)(\widehat{\mathbf{x}}), \tag{67}$$

where we used Eq. (53). Hence,

$$\mathscr{W}^{-1}[f(\mathbf{x})\mathbf{p}] = \frac{1}{2}\left[f(\widehat{\mathbf{x}})\widehat{\mathbf{p}} + \widehat{\mathbf{p}}f(\widehat{\mathbf{x}})\right]. \tag{68}$$

### B. $\mathscr{W}^{-1}[p_\alpha p_\beta f(\mathbf{x})]$

Now, consider

$$\begin{aligned} &\mathscr{W}_z[\widehat{p}_\alpha f(\widehat{\mathbf{x}})\widehat{p}_\beta] = p_\alpha\star f(\mathbf{x})\star p_\beta\\ &= \left[p_\alpha f(\mathbf{x}) - \frac{i}{2}\partial_\alpha f(\mathbf{x})\right]\star p_\beta\\ &= p_\alpha f(\mathbf{x})\left(1+\frac{i}{2}\overleftarrow{\partial}_{\mathbf{x}}\cdot\overrightarrow{\partial}_{\mathbf{p}}\right)p_\beta - \frac{i}{2}\partial_\alpha f(\mathbf{x})\star p_\beta\\ &= p_\alpha p_\beta f(\mathbf{x}) + \frac{i}{2}p_\alpha\partial_\beta f(\mathbf{x}) - \frac{i}{2}\left[\partial_\alpha f(\mathbf{x})p_\beta + \frac{i}{2}\partial^2_{\alpha\beta}f(\mathbf{x})\right]\\ &= p_\alpha p_\beta f(\mathbf{x}) + \frac{i}{2}p_\alpha\partial_\beta f(\mathbf{x}) - \frac{i}{2}p_\beta\partial_\alpha f(\mathbf{x}) + \frac{1}{4}\partial^2_{\alpha\beta}f(\mathbf{x}). \end{aligned}$$

(Again, all but the first terms are due to non-commutation of $\widehat{\mathbf{x}}$ and $\widehat{\mathbf{p}}$ and vanish when the commutator is negligible.) Then,

$$\begin{aligned} \mathscr{W}^{-1}[p_\alpha p_\beta f(\mathbf{x})] &= \widehat{p}_\alpha f(\widehat{\mathbf{x}})\widehat{p}_\beta - \frac{i}{2}\mathscr{W}^{-1}[p_\alpha\partial_\beta f(\mathbf{x})]\\ &\quad + \frac{i}{2}\mathscr{W}^{-1}[p_\beta\partial_\alpha f(\mathbf{x})] - \frac{1}{4}(\partial^2_{\alpha\beta}f)(\widehat{\mathbf{x}}), \end{aligned} \tag{69}$$

where we used Eq. (53). In particular, if $f=\Theta^{\alpha\beta}$ such that $\Theta^{\alpha\beta}=\Theta^{\beta\alpha}$ and summation over repeating indices is assumed, then

$$\mathscr{W}^{-1}[p_\alpha p_\beta\Theta^{\alpha\beta}(\mathbf{x})] = \widehat{p}_\alpha\Theta^{\alpha\beta}(\widehat{\mathbf{x}})\widehat{p}_\beta - \frac{1}{4}(\partial^2_{\alpha\beta}\Theta^{\alpha\beta})(\widehat{\mathbf{x}}),$$

where we used $p_\beta\partial_\alpha\Theta^{\alpha\beta} = p_\alpha\partial_\beta\Theta^{\beta\alpha} = p_\alpha\partial_\beta\Theta^{\alpha\beta}$.

## VII. CONCLUSIONS

The Weyl calculus that is commonly considered for Euclidean configuration spaces is readily generalizable to any curved configuration space diffeomorphic to $\mathbb{R}^n$. As we showed here, the key theorems hold up to metric factors. Moreover, the Moyal product and the Weyl correspondence between operators and their symbols are entirely independent of the metric tensor.


[1] C. Gneiting, T. Fischer, and K. Hornberger, *Quantum phase-space representation for curved configuration spaces*, Phys. Rev. A **88**, 062117 (2013).

[2] I. Y. Dodin, *Geometric view on noneikonal waves*, Phys. Lett. A **378**, 1598 (2014).

[3] E. R. Tracy, A. J. Brizard, A. S. Richardson, and A. N. Kaufman, *Ray Tracing and Beyond: Phase Space Methods in Plasma Wave Theory* (Cambridge University Press, New York, 2014).

[4] D. E. Ruiz, *Geometric theory of waves and its applications to plasma physics*, Ph.D. Thesis, Princeton University (2017), arXiv:1708.05423.

[5] B. S. DeWitt, *Point transformations in quantum mechanics*, Phys. Rev. **85**, 653 (1952).

[6] J. M. Domingos and M. H. Caldeira, *Self-adjointness of momentum operators in generalized coordinates*, Found. Phys. **14**, 147 (1984).

[7] For example, $\bar{g} = 1$ can be adopted. Furthermore, if Eqs. (1) and (2) are formally postulated, the physical meaning of $g$ does not matter either, since the metric tensor is not explicitly used in our calculations.
